# Supplementary material for: A mechanistic framework for a priori pharmacokinetic predictions of orally inhaled drugs
Source: arXiv:2006.05092 ancillary file (2020-06-09)
Supplement: Supplementary file 2 [file S1_Table.pdf]

Table 1 Summary of studies for fluticasone propionate and budesonide<sup>#</sup>

| Drug / substance       | Study No   | Description                      | Population                                          | Device                         | Dose<br>[µg]                                         | Comment                                                                                         | References                                                                      |
|------------------------|------------|----------------------------------|-----------------------------------------------------|--------------------------------|------------------------------------------------------|-------------------------------------------------------------------------------------------------|---------------------------------------------------------------------------------|
| Gold / polystyrene     | 1          | Insoluble mono-disperse particle | Healthy volunteers                                  | “compressed air nebulizer”     | NA                                                   | Insoluble particles to evaluate mucociliary clearance model                                     | Smith et al. (1)                                                                |
| Fluticasone propionate | 2          | Mono-disperse particles          | Asthma patients                                     | Spinning top aerosol generator | 50                                                   | Included to allow direct comparison between different inhaled particle sizes                    | Usmani et al. (2, 3)                                                            |
|                        | 3          | Sandoz Citizen Petition          | Healthy volunteers                                  | Diskus®                        | 100, 250, 500 (in combination with 50 µg Salmeterol) | Geometric mean data of 31 individual batches                                                    | Chrystyn (5), Tarsin et al. (6), Kamin et al. (4), Sandoz Citizen Petition (7)  |
|                        | 4          | PK study                         | Healthy volunteers                                  | Diskus®                        | 200, 500 µg (Single dose and steady state)           | Study, which simultaneously provides budesonide and fluticasone propionate data                 | Möllmann et al. (8)                                                             |
|                        | 5          | PK study (IV + inhaled)          | Healthy volunteers and COPD patients                | pMDI + spacer                  | 1000 µg (both iv + inhaled)                          |                                                                                                 | Singh et al. (9)                                                                |
|                        | 6          | PK study                         | Healthy volunteers and moderately severe asthmatics | Accuhaler®                     | 1000 µg                                              | Clear difference between healthies and asthmatics                                               | Harrison and Tattersfield (10)                                                  |
|                        | 7          | IV PK study                      | Healthy volunteers                                  | NA                             | 250, 500, 1000 µg                                    |                                                                                                 | Mackie et al. (11)                                                              |
|                        | 8          | PK study (IV + inhaled)          | Healthy volunteers and mild asthmatic patients      | Diskus®, pMDI                  | 1000 µg (200 µg IV)                                  | Publication demonstrates that systemic disposition is not different in healthies and asthmatics | Thorsson et al. (12)                                                            |
|                        | 9          | PK study (IV + inhaled)          | Healthy volunteers                                  | Diskhaler®, Diskus®            | 1000 µg (250 µg IV)                                  |                                                                                                 | Mackie et al. (13)                                                              |
|                        | 10         | PK study (inhaled)               | Mild-to-moderate asthmatic patients                 |                                | 100 / 500 µg Diskhaler, 500 µg Diskus®               |                                                                                                 | Falcoz et al. (14)                                                              |
|                        | 11         | IV PK study                      | Healthy volunteers and asthmatic patients           | NA                             | Not provided                                         | Even though asthma and healthy data is available; no difference was investigated                | Källen and Thorsson (15)                                                        |
|                        | Budesonide | 4                                | PK in healthy volunteers                            | Healthy volunteers             | Turbohaler®                                          | 400, 1000 µg (Single dose and steady state)                                                     | Study, which simultaneously provides budesonide and fluticasone propionate data |

|    |                         |                                                     |                  |                     |                                                                                                 |                                |
|----|-------------------------|-----------------------------------------------------|------------------|---------------------|-------------------------------------------------------------------------------------------------|--------------------------------|
| 6  | PK study                | Healthy volunteers and moderately severe asthmatics | Turbohaler®      | 1200 µg             | No relevant difference between healthies and asthmatics                                         | Harrison and Tattersfield (10) |
| 8  | PK study (IV + inhaled) | Healthy volunteers and (mild) asthmatic patients    | Turbohaler®      | 1000 µg (200 µg IV) | Publication demonstrates that systemic disposition is not different in healthies and asthmatics | Thorsson et al. (12)           |
| 12 | PK study (IV + inhaled) | Healthy volunteers                                  | Turbohaler, pMDI | 1000 µg             |                                                                                                 | Thorsson et al. (16)           |
| 11 | IV PK study             | Healthy volunteers and asthmatic patients           | NA               | Not provided        | Even though asthma and healthy data is available; no difference was investigated                | Källén and Thorsson (15)       |

IV: intravenous, NA: not applicable, PK: pharmacokinetics, pMDI: pressurized metered dose inhaler

\* The deposition patterns, which were initially calculated for healthy volunteers based on the MPPD tool, were adapted based on the central/ intermediate to peripheral deposition ratios reported by Usmani et al. for asthmatic patients. FP: Fluticasone propionate, TED: total emitted dose (as % of total nominal dose)

# Green-shaded studies were investigated for model evaluation. Study 1 for evaluation of the deposition and mucociliary clearance model of the overall simulation framework, Study 2 to evaluate the pharmacokinetics after inhalation of different particle sizes with varying aerodynamic particle size, Study 4 to evaluate the predicted pharmacokinetics between budesonide and fluticasone propionate, and Study 6 to compare the predicted pharmacokinetics for both healthy volunteers and asthmatics. Other studies were not considered, as these did not include a comparison of one of the above listed aspects within a single study.

Table 2 PK parameters reported / calculated for the PK studies provided in Table 1

| Drug / substance    | Study No | Description        | PK Parameters                                                                    | Cmax                                                                     |                                         | tmax [min] | AUC          |                                          | Comments                                                                                           | References                                                                     |
|---------------------|----------|--------------------|----------------------------------------------------------------------------------|--------------------------------------------------------------------------|-----------------------------------------|------------|--------------|------------------------------------------|----------------------------------------------------------------------------------------------------|--------------------------------------------------------------------------------|
|                     |          |                    |                                                                                  | Reported Cmax                                                            | Dose-normalized Cmax [nmol/L / mg dose] |            | Reported AUC | Dose-normalized AUC [nmol/L*h / mg dose] |                                                                                                    |                                                                                |
| Gold / poly-styrene | 1        |                    | Profile of particles in the lung over time                                       | Not applicable, gold and styrene particles are mainly not being absorbed |                                         |            |              |                                          |                                                                                                    | Smith et al. (1)                                                               |
| FP                  | 2        | 1.5 µm<br>50 µg    | C <sub>max</sub> , t <sub>max</sub> , AUC <sub>0-12h</sub>                       | 425 pg/mL                                                                | 17.0                                    | 8          | 923 pg/mL*h  | 36.9                                     | Even with 100% lung dose and 100% pulmonary bioavailability, the AUC is still higher than expected | Usmani et al. (2, 3)                                                           |
|                     |          | 3 µm<br>50 µg      |                                                                                  | 278 pg/mL                                                                | 11.1                                    | 19         | 891 pg/mL*h  | 35.6                                     |                                                                                                    |                                                                                |
|                     |          | 6µm<br>50 µg       |                                                                                  | 85.0 pg/mL                                                               | 3.40                                    | 30         | 222 pg/mL*h  | 8.87                                     |                                                                                                    |                                                                                |
|                     | 3        |                    | Dose-normalized C <sub>max</sub> , t <sub>max</sub> , geometric mean PK profiles |                                                                          |                                         |            |              |                                          |                                                                                                    | Chrystyn (5), Tarsin et al. (6), Kamin et al. (4), Sandoz Citizen Petition (7) |
|                     | 4        | 200 µg<br>Day 1    | C <sub>max</sub> , AUC, mean PK profiles                                         | 0.037 ng/mL                                                              | 0.370                                   | 90         | 0.22 ng/mL*h | 2.20                                     |                                                                                                    | Möllmann et al. (8)                                                            |
|                     |          | 200 µg<br>Day 5    |                                                                                  | 0.058 ng/mL                                                              | 0.579                                   | 30         | 0.30 ng/mL*h | 3.00                                     |                                                                                                    |                                                                                |
|                     |          | 500 µg<br>Day 1    |                                                                                  | 0.094 ng/mL                                                              | 0.376                                   | 90         | 0.79 ng/mL*h | 3.16                                     |                                                                                                    |                                                                                |
|                     |          | 500 µg<br>Day 5    |                                                                                  | 0.156 ng/mL                                                              | 0.623                                   | 90         | 0.94 ng/mL*h | 3.76                                     |                                                                                                    |                                                                                |
|                     | 5        | 1000 µg<br>Healthy | C <sub>max</sub> , AUC, mean PK profiles                                         | 421 pg/mL                                                                | 0.841                                   | 45         | 2996 pg/mL*h | 5.99                                     | FP administered with pMDI                                                                          | Singh et al. (9)                                                               |
|                     |          | 1000 µg<br>COPD    |                                                                                  | 235 pg/mL                                                                | 0.469                                   | 45         | 1961 pg/mL*h | 3.92                                     | 44% decreased Cmax and 35% decreased AUC compared to healthies                                     |                                                                                |
|                     | 6        | 1000 µg<br>Healthy | Cmax, AUC, mean PK profiles                                                      | 130 pg/mL                                                                | 0.260                                   | 60-120     | 712 pg/mL*h  | 1.42                                     |                                                                                                    | Harrison and Tattersfield (10)                                                 |

|            |   |                             |                                                                                     |               |       |                                                             |                  |       |                                                                                                                            |                                      |
|------------|---|-----------------------------|-------------------------------------------------------------------------------------|---------------|-------|-------------------------------------------------------------|------------------|-------|----------------------------------------------------------------------------------------------------------------------------|--------------------------------------|
|            |   | 1000 µg<br>Asthmatic        |                                                                                     | 78 pg/mL      | 0.156 | 60-120                                                      | 404<br>pg/mL*h   | 0.807 | 40% decreased Cmax and 43%<br>decreased AUC compared to<br>healthies                                                       |                                      |
| 8          |   | 1000 µg<br>Healthy          | C <sub>max</sub> , AUC,<br>mean PK<br>profiles                                      | 0.5 nmol/L    | 0.5   | 100                                                         | 3.5<br>nmol/L*h  | 3.5   | Complete PK profiles only<br>provided as a summary of<br>healthies and mild asthmatics                                     | Thorsson et al.<br>(12)              |
|            |   | 1000 µg<br>Asthmatic        |                                                                                     | 0.4 nmol/L    | 0.4   | 79                                                          | 3.0<br>nmol/L*h  | 3.0   | Low time points considered as<br>intention to treat (log scale jitter<br>data points?)                                     |                                      |
| 9          |   | 1000 µg<br>Diskus           | C <sub>max</sub> , t <sub>max</sub> ,<br>AUC, mean PK<br>profiles                   | 0.339 µg/L    | 0.677 | 25                                                          | 2.49<br>µg/L*h   | 4.97  | 20% decreased Cmax and 14%<br>decreased AUC compared to<br>healthies                                                       | Mackie et al.<br>(13)                |
| 10         |   | 500 µg Diskus<br>Asthmatics | C <sub>max</sub> , t <sub>max</sub> ,<br>AUC, mean PK<br>profile at steady<br>state | 0.092 µg/L    | 0.368 | 40                                                          | 0.474<br>µg/L*h  | 1.89  | TBD                                                                                                                        | Falcoz et al.<br>(14)                |
| Budesonide | 4 | 500 µg<br>Day 1             | C <sub>max</sub> , AUC,<br>mean PK<br>profiles                                      | 0.45 ng/mL    | 2.09  | 10                                                          | 0.99<br>ng/mL*h  | 4.60  |                                                                                                                            | Möllmann et<br>al.<br>(8)            |
|            |   | 500 µg<br>Day 5             |                                                                                     | 0.48 ng/mL    | 2.23  | 30                                                          | 1.22<br>ng/mL*h  | 5.67  |                                                                                                                            |                                      |
|            |   | 1000 µg<br>Day 1            |                                                                                     | 0.90 ng/mL    | 2.09  | 10                                                          | 2.53<br>ng/mL*h  | 5.88  |                                                                                                                            |                                      |
|            |   | 1000 µg<br>Day 5            |                                                                                     | 1.10 ng/mL    | 2.55  | 20                                                          | 2.98<br>ng/mL*h  | 6.92  |                                                                                                                            |                                      |
| 6          |   | Healthy<br>1200 µg          | C <sub>max</sub> , AUC,<br>mean PK<br>profiles                                      | 2432 pg/mL    | 4.70  | NA                                                          | 6467<br>pg/mL*h  | 12.5  | Dose-normalized AUC and Cmax<br>for healthies ~2 fold higher than<br>reported in Möllmann et al. (at a<br>comparable dose) | Harrison and<br>Tattersfield<br>(10) |
|            |   | Asthmatic<br>1200 µg        |                                                                                     | 2276 pg/mL    | 4.40  | NA<br>(first time<br>point<br>already<br>t <sub>max</sub> ) | 7293<br>pg/mL*h  | 14.1  |                                                                                                                            |                                      |
| 8          |   | 1000 µg<br>Healthy          | C <sub>max</sub> , AUC,<br>mean PK<br>profiles                                      | 3.8<br>nmol/L | 3.8   | 17                                                          | 10.5<br>nmol/L*h | 10.5  |                                                                                                                            | Thorsson et al.<br>(12)              |
|            |   | 1000 µg<br>Asthmatic        |                                                                                     | 4.3<br>nmol/L | 4.3   | 15                                                          | 12.9<br>nmol/L*h | 12.9  |                                                                                                                            |                                      |
| 12         |   | 1000 µg<br>Healthy          | C <sub>max</sub> , AUC,<br>mean PK<br>profiles                                      | NA            | NA    | NA                                                          | 3.5<br>nmol/L*h  | 3.5   | TBD                                                                                                                        | Thorsson et al.<br>(16)              |

## References

1. Smith JR, Bailey MR, Etherington G, Shutt AL, Youngman MJ. Effect of particle size on slow particle clearance from the bronchial tree. *Exp Lung Res.* 2008;34(6):287-312.
2. Usmani OS, editor *Exploring Aerosol Absorption in Humans: Pharmacokinetics of Monodisperse Fluticasone Propionate.* Respiratory Drug Delivery 2014; 2014; Fajardo, Puerto Rico: Davis Healthcare International Publishing, LLC; 2014.
3. Usmani OS, Biddiscombe MF, Barnes PJ. Regional lung deposition and bronchodilator response as a function of  $\beta$ 2-agonist particle size. *American Journal of Respiratory and Critical Care Medicine.* 2005;172(12):1497-504.
4. Kamin WE, Genz T, Roeder S, Scheuch G, Trammer T, Juenemann R, et al. Mass output and particle size distribution of glucocorticosteroids emitted from different inhalation devices depending on various inspiratory parameters. *Journal of aerosol medicine : the official journal of the International Society for Aerosols in Medicine.* 2002;15(1):65-73.
5. Chrystyn H. The Diskus: a review of its position among dry powder inhaler devices. *Int J Clin Pract.* 2007;61(6):1022-36.
6. Tarsin WY, Pearson SB, Assi KH, Chrystyn H. Emitted dose estimates from Seretide Diskus and Symbicort Turbuhaler following inhalation by severe asthmatics. *International journal of pharmaceuticals.* 2006;316(1-2):131-7.
7. A. Maffia G. Sandoz Citizen Petition 2016 [Available from: <https://s3.amazonaws.com/assets.fiercemarkets.net/public/005-LifeSciences/SandozCitizenPetition.pdf>].
8. Möllmann H, Wagner M, Krishnaswami S, Dimova H, Tang Y, Falcoz C, et al. Single-dose and steady-state pharmacokinetic and pharmacodynamic evaluation of therapeutically clinically equivalent doses of inhaled fluticasone propionate and budesonide, given as diskus® or turbuhaler® dry-powder inhalers to healthy subjects. *Journal of clinical pharmacology.* 2001;41(12):1329-38.
9. Singh SD, Whale C, Houghton N, Daley-Yates P, Woodcock AA. Pharmacokinetic and systemic effects of inhaled fluticasone propionate in chronic obstructive pulmonary disease. *British journal of clinical pharmacology.* 2003;55:375-81.
10. Harrison TW, Tattersfield AE. Plasma concentrations of fluticasone propionate and budesonide following inhalation from dry powder inhalers by healthy and asthmatic subjects. *Thorax.* 2003;58(3):258-60.
11. Mackie AE, Ventresca GP, Fuller RW, Bye A. Pharmacokinetics of intravenous fluticasone propionate in healthy subjects. *British journal of clinical pharmacology.* 1996;41(6):539-42.
12. Thorsson L, Edsbacker S, Källén A, Löfdahl C-G. Pharmacokinetics and systemic activity of fluticasone via Diskus(R) and pMDI, and of budesonide via Turbuhaler. *British journal of clinical pharmacology.* 2001;52:529-38.
13. Mackie AE, McDowall JE, Falcoz C, Ventresca P, Bye A, Daley-Yates PT. Pharmacokinetics of fluticasone propionate inhaled via the Diskhaler and Diskus powder devices in healthy volunteers. *Clinical pharmacokinetics.* 2000;39 Suppl 1:23-30.
14. Falcoz C, Horton J, Mackie AE, Harding SM, Daley-Yates PT. Pharmacokinetics of fluticasone propionate inhaled via the Diskhaler and Diskus powder devices in patients with mild-to-moderate asthma. *Clinical pharmacokinetics.* 2000;39 Suppl 1:31-7.
15. Kallen A, Thorsson L. Drug disposition analysis: a comparison between budesonide and fluticasone. *Journal of pharmacokinetics and pharmacodynamics.* 2003;30(4):239-56.

16. Thorsson L, Edsbacker S, Conradson TB. Lung deposition of budesonide from Turbuhaler® is twice that from a pressurized metered-dose inhaler P-MDI. *European Respiratory Journal*. 1994;7(10):1839-44.
